# Supplementary material for: WideSeek: Advancing Wide Research via Multi-Agent Scaling
Source: arXiv:2602.02636 source file (2026-02-02)
Supplement: Supplementary file 1 [file appendix.tex]

\input{content/appendix/wideseekbench}
